# Supplementary material for: Building a Chinese Medical Dialogue System: Integrating Large-scale Corpora and Novel Models
Source: arXiv:2410.03521 source file (2025-02-25)
Supplement: Supplementary file 1 [file 10-appendix.tex]

\section{Dataset Details}

\section{Discussion}
\label{app:diss}

\subsection{Data Issues}
During data collection, we found certain biases in the data gathered from online platforms. Firstly, acute and severe cases are not typically presented online, as patients in these situations usually go directly to the hospital. Secondly, the internet acts as a filter, with the online population differing from the general population. This results in a majority of younger users seeking online consultations, leading to a lack of data on elderly conditions. Lastly, due to the anonymity of the internet, the nature of questions asked online can differ from those asked offline, often including more private issues.

Medical issues require maximum caution, and licensed doctors undergo extensive training to earn their qualifications due to the severe consequences of medical errors, which can endanger lives. Therefore, using current AI, which often functions as a black-box system, for diagnosis and treatment remains an ethical and legal grey area. At present, AI can only serve as a supplementary tool. Similar to autonomous driving, where accidents pose challenges in accountability, AI in healthcare must develop gradually. Automation systems must advance in a phased manner.

\subsection{Discussion on Current Large Models}
With the rise of ChatGPT, pre-trained language models seem to have deviated from their original purpose but have unified various tasks. Previously proposed task classifications are now outdated. Since the introduction of the T5 model, all-natural language processing tasks can be modeled as text generation tasks, differing only in prompts. Currently, the boundaries between various big data tasks are unclear, and many tasks can be converted into generative tasks. 
The popularity of ChatGPT has even given rise to a new role, "prompt engineer," who specializes in crafting effective prompts to leverage ChatGPT for task completion. 
In the future, large models can liberate and enhance productivity, handling repetitive tasks and freeing humans for creative work, thus advancing technological progress. 

\subsection{Comparison Between Industrial and Research Institutions in Large Model Development}
Industries aim to generate profits, driving them to develop market-appropriate large models with high enthusiasm. They also have vast user bases that provide data and accelerate training. However, industries face ethical and legal constraints, such as patents and privacy issues. Research institutions, lacking immediate application needs or access to first-hand data, face disadvantages in a data-driven era. Nonetheless, they pursue innovation without profit motives, experimenting in numerous directions, where even a one-in-a-million success marks a significant breakthrough. Furthermore, research institutions frequently refresh their teams, maintaining high efficiency in research.

% \section{Potential Future Work}
% \label{app:futurework}

% \subsection{Dataset Extension}
% Collecting data from multiple sources can help mitigate the bias faced in the dataset.

% \subsection{Intelligent Triage}
% The All-in-one LLMs can solve the triage in a more general way. Researchers may pay more attention to adding more background information, such as multi-modality methods. Double checking will ground truth after the decision is also important due to the high risk of medical problems.

% \subsection{Medical Consultant}
% Medical consultation systems have a promising future as AI technology advances, with human resources and potentially unlimited computing resources that can scale with demand. With the development of current LLMs, constructing a consultation system become easier. Researchers can shift their focus to the alignment between LLM output and human preference (legal issues, correct knowledge, cost trade-off). The RLHF may contribute to the alignment.

% \subsection{Further Application}
% The power of LLMs may empower more complicated tasks. As a result, researchers may not need to formulate real tasks into fixed mathematical tasks, which will enable more flexible and realistic solutions. Researchers may extend the usage of our datasets based on their own need.
